# Supplementary material for: State-of-the-art generalisation research in NLP: A taxonomy and review
Source: arXiv:2210.03050 source file (2024-01-12)
Supplement: Supplementary file 1 [file appendix_FAQ.tex]

\section{Annotation FAQ}\label{appendix:FAQ}

\begin{itemize}

\item Does using masked language modeling as the pretraining objective imply that there is a covariate shift from pretraining to finetuning, given that all pretraining inputs contain special masked tokens and finetuning inputs do not?

\item Even when leaving masking aside, isn't there always a covariate shift between pretraining and finetuning? The opposite would imply that random samples from the pretraining corpus would be indistinguishable from those from the downstream task. Even if there is data leakage this will never be the case in practice, as the leaked data will be mixed with other content in the pretraining corpus and their distribution will therefore not be strictly the same.

\item If no new parameters are added for finetuning, does that imply that there is no label shift? How should we annotate T5 and similar approaches?

\item When a pretrained language model is evaluated on language modeling itself, is the locus pretrain-test or train-test?

\end{itemize}
